# Supplementary material for: StepGame: A New Benchmark for Robust Multi-Hop Spatial Reasoning in Texts
Source: arXiv:2204.08292 source file (2022-04-18)
Supplement: Supplementary file 1 [file appendix.tex]

\section{Test Accuracy on the Noise-Free StepGame Dataset}
\begin{table*}[!t]
% \footnotesize
\begin{adjustbox}{max width=\textwidth}
\begin{tabular}{lrrrrrr}
\hline
\hline
%\multicolumn{7}{c}{Test Accuracy for StepGame}                                                                                     %                                                    \\ \hline
Models & 
\multicolumn{1}{c}{$k=1$} & 
\multicolumn{1}{c}{$k=2$} & 
\multicolumn{1}{c}{$k=3$} & 
\multicolumn{1}{c}{$k=4$} & 
\multicolumn{1}{c}{$k=5$} & 
\multicolumn{1}{c}{Mean}           \\ \hline
RN~\cite{santoro2017simple}       & 44.43$\pm$4.00          & 33.20$\pm$3.65           & 23.74$\pm$2.35           & 17.90$\pm$1.15          & 14.80$\pm$2.41         & 26.81          \\
RRN~\cite{palm2018recurrent}      & 45.98$\pm$5.18          & 35.94$\pm$2.48           & 26.90$\pm$1.91           & 18.52$\pm$1.50          & 15.54$\pm$1.50         & 28.58          \\
UT~\cite{dehghani2018universal}   & 65.21$\pm$3.23          & 38.22$\pm$2.20           & 26.56$\pm$2.37           & 22.50$\pm$2.62          & 16.58$\pm$2.63         & 33.81          \\
STM~\cite{le2020self}             & 60.09$\pm$4.34          & 47.02$\pm$2.41           & 35.25$\pm$2.50           & 24.43$\pm$2.10          & 21.44$\pm$3.02         & 37.65          \\
TPR-RNN~\cite{schlag2018learning} & 90.08$\pm$2.38          & 58.26$\pm$3.77           & 45.72$\pm$3.83           & 34.70$\pm$4.48          & 29.30$\pm$3.07         & 51.61          \\\hline
TP-MANN                          & \textbf{96.98$\pm$0.20}  & \textbf{72.30$\pm$1.35} & \textbf{57.68$\pm$1.18} & \textbf{48.56$\pm$1.83} & \textbf{42.28$\pm$1.98} & \textbf{63.56} \\
\hline
\hline
\end{tabular}
\end{adjustbox}
\caption{Test accuracy on StepGame: Mean$\pm$Std over 5 runs. $k$ represents the size of the story.}% For each model, we use random seeds to run 10 times and average the best 5 results.}
\label{tbl:step_game}
\end{table*}

We test the all the baselines and our model on a noise-free version of the StepGame dataset. The results are shown in Table~\ref{tbl:step_game} where we break down the performance of the trained models per $k$. In the last column we report the average performance across $k$.

Our model outperforms all baseline models on all five tasks, while TPR-RNN achieves the best performance among the baselines. The performance of all baseline models decreases when the number of required inference hops $k$ increases. 

\section{Statistics of Distracting Noise}
\begin{table}[!th]
\centering
\small
\begin{adjustbox}{max width=\textwidth}
\begin{tabular}{l|lllll}
\hline
\hline
Noise Type & $k$=1 & $k$=2 & $k$=3 & $k$=4 & $k$=5 \\ \hline 
Supporting & 0.0 & 0.0 & 0.0 & 1.4 & 1.6 \\
Disconnected & 2.0 & 2.0 & 2.0 & 2.0 & 2.5 \\
Irrelevant & 1.0 & 1.5 & 1.5 & 1.5 & 2.0 \\ \hline
Total & 3.0 & 3.5 & 3.5 & 4.9 & 6.1 \\ \hline \hline
Noise Type & $k$=6 & $k$=7 & $k$=8 & $k$=9 & $k$=10 \\ \hline
Supporting & 1.7 & 1.9 & 2.0 & 2.1 & 2.1 \\
Disconnected & 2.5 & 2.5 & 3.0 & 3.0 & 3.0 \\
Irrelevant & 2.0 & 2.0 & 2.5 & 2.5 & 2.5 \\ \hline
Total & 6.3 & 6.4 & 7.5 & 7.6 & 7.6 \\ \hline \hline
\end{tabular}
\end{adjustbox}
\label{statistics}
\caption{The average number of nodes used for each type of distracting noise.}
\end{table}

In Table 2, we present the statistics of distracting noise of test sets. We only add supporting noise for test sets whose $k$ is larger than 2. It is worth noting that the number of nodes used for disconnected noise is larger than that for irrelevant nodes. This is because when the number of noise sentences is the same, disconnected noise uses one more nodes than irrelevant nodes.

\section{Training Details of TP-MANN on the StepGame Dataset}
We examine our TP-MANN model on the StepGame dataset. Each story is pre-processed into a sentence-level sequence. The story and its corresponding question will be treated as inputs. Then, we utilize the TP-MANN to compute a probability distribution over the vocabulary $\*V$. TP-MANN’s hyper-parameters are fixed to $d$=256, $d_e$=200, $d_r$=80, the recurrent layer is 8, the dimension of hidden layers in MLPs are all set to 200. We train our model jointly for 5 tasks ($k$=1,2,3,4,5) with a cross entropy loss function and a batch size of 50, using Adam as the optimizer~\cite{kingma2014adam} with a learning rate of 0.001, $\beta_1$ = 0.9 and $\beta_2$ = 0.99. We select the best model based on the validation set. The total parameters size is 4.0M. The hyperparameters of TP-MANN on the bAbI dataset follows the same settings as above.
% Details of all runs are listed in Table \ref{}.

\section{Implementation Details of Baselines on the StepGame Dataset}
\label{hyper_stepgame}
\textbf{Setup} For all models, we use the same encoder in the TP-MANN to encode stories $S=(s_1, \dots, s_m)$ with $m$ sentences and a question $q$, and feed them into each baseline. All baselines return a softmax distribution over the vocabulary $\*V$. We use Adam as the optimizer~\cite{kingma2014adam} for all models. All baseline models are trained under a joint training setting. We use the validation sets to tune the optimal hyperparameters for all baselines, based on the validation accuracy. We conducted 10 runs with different initializations and picked the best 5 runs based on the performance on the validation set. Hyper-parameter settings are listed in Table \ref{rRn_hpyer}, \ref{rn_hpyer}, \ref{TPR_hpyer}, \ref{stm_hpyer}, and \ref{ut_hpyer} respectively. The values we finally adopted are in bold. %Note that we do not tune all the hyperparameters.

\textbf{Recurrent Relational Networks}~\cite{palm2018recurrent} To map the questions into a graph we treat each sentence related to a question as the nodes. In the table \ref{rRn_hpyer}, $LSTM_S$ and $LSTM_Q$ refer to the LSTM for story and question respectively. Different from the original paper, we do not add a random offset $o$ to each node feature vector to make the tasks easier. Message Size refers to $m^t_j$ in the original paper. $MLP_1$, $MLP_2$, and $MLP_3$ refer to the input MLP, message MLP, and output MLP respectively. We experimented with different hyper-parameters and different network sizes, but unfortunately none of them can converge even when the value of $k=1$. Our implementation is based on an open source implementation\footnotemark.
\begin{table}[!th]
\centering

% \small
% \normalsize	
% \begin{adjustbox}{max width=\textwidth}
\footnotesize
\begin{tabular}{p{4.9cm}r}
\hline
\hline
\textbf{Hyperparameters} & \textbf{Value} \\ \hline
Batch Size & 100, \textbf{500}, 2000 \\
Learning Rate & 1e-5, \textbf{1e-4}, 1e-3 \\
Epoch & \textbf{1500} \\
Word Embedding Size & 32, \textbf{64} \\
Hidden Size of $LSTM_S$ & 32, \textbf{64} \\
Hidden Size of $LSTM_Q$ & 32, \textbf{64} \\
Hidden Size of $LSTM_G$ & \textbf{128}, 256 \\
Hidden Size of $MLP_1$ & 128, \textbf{256}, 512 \\
Hidden Size of $MLP_2$ & 128, \textbf{256}, 512 \\
Hidden Size of $MLP_3$ & 128, \textbf{256}, 512 \\
Activation Function & \textbf{ReLU}, Tanh \\
Message Size & \textbf{128}, 256 \\
Dropout & \textbf{0.5} \\ \hline
Numbers of Parameters & \textbf{1.1M} \\ \hline
\hline
\end{tabular}
% \end{adjustbox}
\caption{Settings for Recurrent Relational Networks (RRN).}
\label{rRn_hpyer}
\end{table}

\textbf{Relation Networks}~\cite{santoro2017simple} An relation module (implemented as an MLP) is used alongside the encoder module to learn pairwise relations among all the pairs of sentences. In Table \ref{rn_hpyer}, $g$ and $f$ refers to MLPs as in the original paper. Our implementation is based on an open source implementation\footnotemark[\value{footnote}].
\footnotetext{\url{https://github.com/AndreaCossu/Relation-Network-PyTorch}}
\begin{table}[h!]
\centering

\footnotesize
\begin{tabular}{p{5.3cm}r}
\hline
\hline
\textbf{Hyperparameters} & \textbf{Value} \\ \hline
Batch Size & \textbf{500} \\
Learning Rate & 1e-4, \textbf{1e-3} \\
Epoch & \textbf{1500} \\
Word Embedding Size & 32, \textbf{64} \\
Hidden Size of g & 256, \textbf{512} \\
Output Size of g & 256, \textbf{512} \\
Hidden Size of f & 256, \textbf{512} \\
Activation Function & \textbf{ReLU}, Tanh \\ \hline
Numbers of Parameters & \textbf{1.5M} \\ \hline
\hline
\end{tabular}
\caption{Settings for Relation Network (RN).}
\label{rn_hpyer}
\end{table}

\textbf{TPR-RNN}~\cite{schlag2018learning} Each sentence in a story is encoded as a vector and fed into the TPR-RNN. In Table \ref{TPR_hpyer}, we follow the default setting as in the original paper. The experiments showed that increasing model's size is not useful to improve the performance of this model. Our implementation is based on an open source implementation\footnote{\url{https://github.com/APodolskiy/TPR-RNN-Torch/tree/master/tpr_rnn}}.
\begin{table}[!th]
\centering

\footnotesize
\begin{tabular}{p{5.6cm}r}
\hline
\hline
\textbf{Hyperparameters} & \textbf{Value}      \\ \hline
Batch Size               & \textbf{500}, 2000  \\
Learning Rate            & 1e-4, \textbf{1e-3} \\
Epoch                    & \textbf{300}, 500   \\
Word Embedding Size      & \textbf{256}     \\
Entity Size              & 60, \textbf{100}    \\
Hidden Size of MLP       & \textbf{100}     \\
Relation Size            & \textbf{50}0 \\ \hline
Numbers of Parameters    & \textbf{381K}     \\ \hline
\hline
\end{tabular}
% \end{adjustbox}
\caption{Settings for TPR-RNN.}
\label{TPR_hpyer}
\end{table}

\textbf{Self-Attentive Associative Memory}~\cite{le2020self} Each sentence in a story is encoded as a vector and fed into the STM. We follow the original paper's setting to treat $\alpha_1$ as 1, $\alpha_2$ as a trainable parameter, and $\alpha_3$ as 0. The entity size, role size, and key size refer to $d$, $n_q$, and $n_{kv}$ respectively as in the original paper. The value of hyperparameters is list in Table \ref{stm_hpyer}. Our implementation is based on an open source implementation\footnote{\url{https://github.com/thaihungle/SAM}}.
\begin{table}[!th]\centering
\footnotesize
\begin{tabular}{p{5cm}r}
\hline
\hline
\textbf{Hyperparameters} & \textbf{Value}          \\ \hline
Batch Size               & 200, \textbf{500}, 1000 \\
Learning Rate            & 1e-4, \textbf{1e-3}  \\
Epoch                    & \textbf{300}, 500       \\
Word Embedding Size      & 128, \textbf{256}    \\
Entity Size          & \textbf{90}             \\
Role Size          & \textbf{20}             \\
Key Size        & \textbf{20}             \\
Weight $\alpha_1$               & \textbf{1}              \\
Weight $\alpha_3$               & \textbf{0}              \\ \hline
Numbers of Parameters    & \textbf{1.5M}           \\ \hline
\hline
\end{tabular}
% \end{adjustbox}
\caption{Settings for Self-Attentive Associative Memory (STM).}
\label{stm_hpyer}
\end{table}

\begin{table}[ht!]
\centering
% \begin{adjustbox}{max width=\textwidth}
\footnotesize
\begin{tabular}{p{5.1cm}r}
\hline
\hline
\textbf{Hyperparameters} & \textbf{Value} \\ \hline
Batch Size & 500, \textbf{1000} \\
Learning Rate & 1e-4, \textbf{1e-3} \\
Epoch & \textbf{2000} \\
Word Embedding Size & 128, \textbf{256} \\
Total Heads & 2, 4, \textbf{8} \\
Depth Size & 512, \textbf{1024} \\
Filter Size &  512, \textbf{1024} \\
Max Hops & \textbf{12} \\ \hline
Numbers of Parameters & \textbf{2.7M} \\ \hline
\hline
\end{tabular}
% \end{adjustbox}
\caption{Settings for Universal Transformer(UT).}
\label{ut_hpyer}
\end{table}
\textbf{Universal Transformer}~\cite{dehghani2018universal} In Table \ref{ut_hpyer}, we use the encoder of UT with a dynamic ACT halting mechanism as the setting in the original paper on the bAbI dataset. Each sentence in a story is encoded as a vector and concatenated with the question vectors. Then we feed them into the UT. The filter size refers to the hidden size of the middle layer in the feed forward layer. The depth size refers to both the dimension of keys and values. The max hops refers to the maximum number of computational steps for dynamic halting. Our implementation is based on an open source implementation\footnote{\url{https://github.com/andreamad8/Universal-Transformer-Pytorch}}.
